# Supplementary material for: SaludConectaMX: Lessons Learned from Deploying a Cooperative Mobile Health System for Pediatric Cancer Care in Mexico
Source: arXiv:2408.00881 source file (2024-08-01)
Supplement: Supplementary file 1 [file 8_Supplementary.tex]

\section{Supplementary Materials}

\subsection{Technical Implementation}
Our web and mobile applications share a common API backend written in Python as a Flask web service hosted in a secure AWS EC2 instance configured to host patient-identifiable information. Access to the EC2 instance is restricted using Okta authentication via Amazon AppStream. Calls to the API are further secured by ensuring the call originated from a logged in user from the web or mobile app. We use PostgreSQL for our database which stores all form data across the patient trajectory (Figure \ref{fig:system}). The patient-facing mobile portion of the application was built with the cross-platform framework Flutter using the Dart programming language and communicates with the same Flask API as the HWA. We chose Flutter to be able to write applications for both iOS and Android. Visuals of both interfaces are shown in Supplementary Figure \ref{fig:interfaces}

\captionsetup{width=\textwidth}

\begin{figure}[H]
  \centering
  \includegraphics[width=.95\columnwidth]{Figures/Dual_Interfaces_HighRes.jpeg}
  \caption{Visuals of the SaludConectaMX Hospital Web Application (left) and Family Mobile Application (right)}
  \Description{An image displaying the SaludConectaMX Hospital Web application. On the left is an image of the main dashboard and on the right is an image of a patient's file.}
  \label{fig:interfaces}
\end{figure}

\subsection{Demographics}

\subsubsection{Enrolled Patients} Of the 274 enrolled patients, 165 (60.2\%) were male and 109 (39.8\%) were female. The age range of patients at the time of enrollment was between 0.10 and 19.76 years (IQR: 4.95 - 12.34 years).

\subsubsection{MARS Respondents} Of the 18 respondents, 4 (22.2\%) were male and 14 (77.8\%) were female. The average age of the survey respondents was 24.4 years (IQR: 24.0 - 25.0). Of the 18 respondents, 1 (5.6\%) completed their master’s degree, 1 (5.6\%) has an incomplete master’s degree, 8 (44.4\%) completed their bachelor’s degree, 6 (33.3\%) have an incomplete bachelor’s degree, and 2 (11.1\%) completed high school. 

\subsection{FMA Missingness Statistics}

Supplementary Figure \ref{fig:enroll} shows patient enrollment throughout the pilot phase, separated into key stages (i.e., HWA deployment, FMA deployment, and FMA assistance). Upon statistical investigation (permutation tests), we do not observe a significant difference in the average number of FMA forms completed between patients enrolled pre- vs. post- FMA deployment ($p=0.843$), which occurred 4 months after the HWA was deployed; this finding remains consistent after excluding patients who enrolled after healthcare staff began to assist with FMA completion ($p=0.797$). Similarly, we do not find that help from healthcare staff significantly contributed to lower average missingess per patient ($p=0.815$), even after excluding patients who enrolled before FMA deployment ($p=0.546$). This finding motivates the need to investigate additional reasons for missingness.

\begin{figure}[h]
    \centering
    \includegraphics[width=0.95\linewidth]{Figures/enrollment_timeline.png}
    \caption{SaludConectaMX patient enrollment, broken down into key stages of the pilot phase.}
    \Description{An image displaying patient enrollment throuughout the key stages of the pilot phase study.}
    \label{fig:enroll}
\end{figure}

\begin{table}[h]
\resizebox{\linewidth}{!}{%
\begin{tabular}{clllll}
\cline{1-3}
\multicolumn{1}{|l|}{\textbf{Interviewee}}                                                                         & \multicolumn{1}{l|}{\textbf{Barrier Description}}                                                                                                                                                                                                                                 & \multicolumn{1}{l|}{\textbf{System Recommendation}}                                                                                                                                                                                                                                                                                                    &  &  &  \\ \cline{1-3}
\multicolumn{1}{|c|}{\multirow{5}{*}{\begin{tabular}[c]{@{}c@{}}Social \\ Worker\end{tabular}}}                    & \multicolumn{1}{l|}{\begin{tabular}[c]{@{}l@{}}(HWA) A limited number of healthcare staff are available for system \\ data collection; medical residents without much system experience \\ were recruited to collect data.\end{tabular}}                                          & \multicolumn{1}{l|}{\begin{tabular}[c]{@{}l@{}}More thorough training for system users will help reduce \\ data collection challenges and biases.\end{tabular}}                                                                                                                                                                                        &  &  &  \\ \cline{2-3}
\multicolumn{1}{|c|}{}                                                                                             & \multicolumn{1}{l|}{\begin{tabular}[c]{@{}l@{}}(FMA) Caregivers experience fatigue when answering the same \\ questions repeatedly throughout the system.\end{tabular}}                                                                                                           & \multicolumn{1}{l|}{\begin{tabular}[c]{@{}l@{}}Eliminate repeated questions across multiple forms in the app. \\ Add additional logic that eliminates cascading questions if \\ certain information is not applicable for the caregiver.\end{tabular}}                                                                                                 &  &  &  \\ \cline{2-3}
\multicolumn{1}{|c|}{}                                                                                             & \multicolumn{1}{l|}{\begin{tabular}[c]{@{}l@{}}(FMA) Caregivers are less interested in participating if they have \\ had a poor experience with physicians (e.g., rude interactions).\end{tabular}}                                                                               & \multicolumn{1}{l|}{\begin{tabular}[c]{@{}l@{}}Healthcare staff will help build positive rapport with families \\ and introduce them to the benefits of the system for their child's \\ wellbeing.\end{tabular}}                                                                                                                                       &  &  &  \\ \cline{2-3}
\multicolumn{1}{|c|}{}                                                                                             & \multicolumn{1}{l|}{\begin{tabular}[c]{@{}l@{}}(FMA) Caregivers do not feel they are compensated for their data\\ collection efforts. They also do not observe any direct benefits from \\ using the system.\end{tabular}}                                                        & \multicolumn{1}{l|}{\begin{tabular}[c]{@{}l@{}}Small financial compensation will be provided, in addition to \\ more helpful app features that incentivize use.\end{tabular}}                                                                                                                                                                          &  &  &  \\ \cline{2-3}
\multicolumn{1}{|c|}{}                                                                                             & \multicolumn{1}{l|}{\begin{tabular}[c]{@{}l@{}}(FMA) Caregivers often answer form questions only with respect to \\ the patient and not with respect to themselves (e.g., food security \\ often does not reflect sacrifices that parents make for their children).\end{tabular}} & \multicolumn{1}{l|}{\begin{tabular}[c]{@{}l@{}}Adding further specifications for certain form questions will \\ ensure better data quality.\end{tabular}}                                                                                                                                                                                              &  &  &  \\ \cline{1-3}
\multicolumn{1}{|c|}{\multirow{4}{*}{\begin{tabular}[c]{@{}c@{}}Medical \\ Residents\end{tabular}}}                & \multicolumn{1}{l|}{\begin{tabular}[c]{@{}l@{}}(HWA + FMA) Internet access is often limited both inside and outside \\ the hospital, making it difficult to submit forms.\end{tabular}}                                                                                           & \multicolumn{1}{l|}{\begin{tabular}[c]{@{}l@{}}Adding modems within the hospital may resolve this issue for\\ the hospital staff.\end{tabular}}                                                                                                                                                                                                        &  &  &  \\ \cline{2-3}
\multicolumn{1}{|c|}{}                                                                                             & \multicolumn{1}{l|}{\begin{tabular}[c]{@{}l@{}}(FMA) Caregivers often forget appointments and forget to fill out \\ forms. Others only use the system when they perceive that their child \\ has a possible risk for a complication event.\end{tabular}}                          & \multicolumn{1}{l|}{\begin{tabular}[c]{@{}l@{}}Additional system features such as reminders and appointment \\ scheduling may assist and incentivize usage. Incorporating a \\ chat bot may also resolve doubts. Caregivers may also benefit \\ from education (via demonstration video) about the importance \\ of the form completion.\end{tabular}} &  &  &  \\ \cline{2-3}
\multicolumn{1}{|c|}{}                                                                                             & \multicolumn{1}{l|}{\begin{tabular}[c]{@{}l@{}}(HWA + FMA) Patients and their caregivers often require medical \\ assistance during the journey to the hospital once symptoms of a \\ complication begin.\end{tabular}}                                                           & \multicolumn{1}{l|}{\begin{tabular}[c]{@{}l@{}}Adding functionalities that allow for communication between \\ caregivers and hospital staff will assist with emergency events \\ (e.g., WhatsApp). An emergency button to notify the hospital \\ about incoming patients would also benefit the care team.\end{tabular}}                               &  &  &  \\ \cline{2-3}
\multicolumn{1}{|c|}{}                                                                                             & \multicolumn{1}{l|}{\begin{tabular}[c]{@{}l@{}}(HWA) Some fields are left blank in the emergency forms and are \\ only filled at a later time, which introduces data biases.\end{tabular}}                                                                                        & \multicolumn{1}{l|}{\begin{tabular}[c]{@{}l@{}}Additional training may ensure that the emergency staff \\ completes all fields at the proper time points.\end{tabular}}                                                                                                                                                                                &  &  &  \\ \cline{1-3}
\multicolumn{1}{|c|}{\multirow{5}{*}{\begin{tabular}[c]{@{}c@{}}Participating \\ Caregivers\end{tabular}}}         & \multicolumn{1}{l|}{\begin{tabular}[c]{@{}l@{}}(FMA) Caregivers expressed they they feel uncomfortable taking \\ vital signs. As a result, they do not collect this information.\end{tabular}}                                                                                    & \multicolumn{1}{l|}{Additional education and training is needed to support.}                                                                                                                                                                                                                                                                           &  &  &  \\ \cline{2-3}
\multicolumn{1}{|c|}{}                                                                                             & \multicolumn{1}{l|}{\begin{tabular}[c]{@{}l@{}}(FMA) Caregivers reflect that they did not consider using the app \\ until their child experienced an emergency event.\end{tabular}}                                                                                               & \multicolumn{1}{l|}{\begin{tabular}[c]{@{}l@{}}Additional education and training is needed to support. \\ Additionally, communication between residents and families \\ could be strengthened.\end{tabular}}                                                                                                                                           &  &  &  \\ \cline{2-3}
\multicolumn{1}{|c|}{}                                                                                             & \multicolumn{1}{l|}{\begin{tabular}[c]{@{}l@{}}(FMA) Caregivers express uncertainty as to whether or not \\ information they entered has been properly logged in the system.\end{tabular}}                                                                                        & \multicolumn{1}{l|}{\begin{tabular}[c]{@{}l@{}}Need better system design / functionality to confirm that the\\ information was logged properly after form submission, in \\ addition to more app training.\end{tabular}}                                                                                                                               &  &  &  \\ \cline{2-3}
\multicolumn{1}{|c|}{}                                                                                             & \multicolumn{1}{l|}{(FMA) Insufficient mobile credit prevents frequent data collection.}                                                                                                                                                                                          & \multicolumn{1}{l|}{\begin{tabular}[c]{@{}l@{}}The research team will work on a plan to provide mobile \\ credit funds to families for data collection.\end{tabular}}                                                                                                                                                                                  &  &  &  \\ \cline{2-3}
\multicolumn{1}{|c|}{}                                                                                             & \multicolumn{1}{l|}{\begin{tabular}[c]{@{}l@{}}(FMA) Most app functionalities are not explained at the time the app\\ is downloaded at the hospital (e.g., some caregivers had no awareness\\ of the mental health pamphlets available within the app).\end{tabular}}             & \multicolumn{1}{l|}{\begin{tabular}[c]{@{}l@{}}Better communication and training between social workers \\ and caregivers is needed to close this gap.\end{tabular}}                                                                                                                                                                                   &  &  &  \\ \cline{1-3}
\multicolumn{1}{|c|}{\multirow{3}{*}{\begin{tabular}[c]{@{}c@{}}Non- \\ Participating \\ Caregivers\end{tabular}}} & \multicolumn{1}{l|}{\begin{tabular}[c]{@{}l@{}}(FMA) Caregivers express that they understand what an emergency \\ event looks like and do not believe the app will provide added support.\end{tabular}}                                                                           & \multicolumn{1}{l|}{\begin{tabular}[c]{@{}l@{}}Add functionalities that incentivize use of the app beyond \\ emergency event recognition.\end{tabular}}                                                                                                                                                                                                &  &  &  \\ \cline{2-3}
\multicolumn{1}{|c|}{}                                                                                             & \multicolumn{1}{l|}{\begin{tabular}[c]{@{}l@{}}(FMA) Caregivers express that instructions for care at home are not \\ always clear. Written instructions from physicians would be helpful.\end{tabular}}                                                                           & \multicolumn{1}{l|}{\begin{tabular}[c]{@{}l@{}}Provide functionality that allows physicians to record detailed \\ care instructions so that caregivers can reference them at home.\end{tabular}}                                                                                                                                                       &  &  &  \\ \cline{2-3}
\multicolumn{1}{|c|}{}                                                                                             & \multicolumn{1}{l|}{\begin{tabular}[c]{@{}l@{}}(FMA) Some caregivers had no knowledge of the app until late in \\ their child's diagnosis / treatment.\end{tabular}}                                                                                                              & \multicolumn{1}{l|}{\begin{tabular}[c]{@{}l@{}}Provide hospital staff with clarification on patient inclusion \\ criteria for system use.\end{tabular}}                                                                                                                                                                                                &  &  &  \\ \cline{1-3}
\multicolumn{1}{l}{}                                                                                               &                                                                                                                                                                                                                                                                                   &                                                                                                                                                                                                                                                                                                                                                        &  &  &  \\
\multicolumn{1}{l}{}                                                                                               &                                                                                                                                                                                                                                                                                   &                                                                                                                                                                                                                                                                                                                                                        &  &  & 
\end{tabular}%
}
\caption{Barrier findings from unstructured interviews with healthcare staff and caregivers.}
\label{tab:interviews}
\end{table}
